# Supplementary material for: Accurate and Fast Approximate Graph Pattern Mining at Scale
Source: arXiv:2405.03488 source file (2024-05-06)
Supplement: Supplementary file 1 [file appendix.tex]

\appendix

\section{Appendix}

\subsection{Lower Bound for Graph Sparsification} \label{subsect:read-k}

Formally, let $Y_1 \dots Y_C$ be the random variables that represent the existence of matches, where $Y_i = 1$ if the match $M_i$ was preserved in the sparsified graph and $Y_i = 0$ if any of the edges within the match were removed.
As $Y_i$ is not independent, this means that we can not use the standard Chernoff bound to tightly bound error. We could use Chebyshev bound 
%(if we consider the covariance between each instance of the pattern in our calculation of the variance), 
but this is not a tight enough bound to be useful in practice. 

We use the `read-$k$' extension of Chernoff bounds~\cite{read-k}. 
The key idea is to map the dependent random variables $Y_i$ to a set of independent random variables $X_i$, and derive a bound from them.
The `read-$k$' extension gives the same bound as that of the standard Chernoff bound, except that the exponent is divided by $k$, where $k$ is the maximum number of $Y_i$ mapped to any $X_j$.

In our case, the edges are removed randomly. 
Let $X_1 \dots X_m$ be random variables for each of the $m$ edges in \dg, where $X_i = 1$ if the edge was preserved and $X_i = 0$ if the edge was removed. We can see each edge has the probability $\hat{p}$ of being preserved and this probability is independent of any other edge, $X_j$, even if they may share one endpoint.
Then $Y_i$ is dependent on exactly $l$ of the $X_1 \dots X_m$ edges, which are the specific edges that make up that match $M_i$. 
We define $\gamma$ as the maximum number of matches (of \pg) incident to an edge.
Thus, we can apply the `read-$k$' extension with $k = \gamma$, which gives the following theorem. 

\begin{theorem}
Given a data graph \dg and a pattern \pg, 
$p \geq \frac{-3\cdot\ln(\delta / 2)\gamma}{\epsilon^2 \cdot C }$
obtains an $\epsilon$-$\delta$ estimation of $C$, the number of matches of \pg in \dg.
\end{theorem}

So in order to determine a good value for $p$, we need to estimate $C$ and $\gamma$,
which is done by the fast profiling~\cref{subsect:profiler} on the graph \dg.
We assume that $\hat{p}$ is not very sensitive to $C$ and $\gamma$. So we don't need a very accurate estimation of $C$ and $\gamma$ in this profiling.

\subsection{Code Examples for \NS-base and Exact GPM} \label{subsect:more-code-example}

\cref{algo:ns-4cycle} shows the pseudo code for neighbor sampling on the \texttt{4-cycle} pattern.

\cref{algo:graphzero-4cycle} shows the pseudo code for neighbor sampling on the \texttt{4-cycle} pattern.

\begin{algorithm}[htb]
\footnotesize
\caption{\NS-base for \texttt{4-cycle}}
\label{algo:ns-4cycle}
\begin{algorithmic}[1]

\For{{\bf each} sampler $i \in$ [1, $N_s$]} \label{algo:ns:line:each-sampler}

%\State $C_i \gets 0$  
\State $e(v_0, v_1) \gets$  \Call{sample}{$\mathcal{E}$} , $\alpha \gets 0$ \Comment{\hlg{sample} an edge $(v_0, v_1)$} \label{algo:ns-base:line:sample-first-edge}
%\State $S_1 \gets$ \{$v_0$, $v_1$\}
\State $A \gets$ $N(v_0) \cup N(v_1)$ - \{$v_0$, $v_1$\}
\Comment{\hlg{set union and difference}}  \label{algo:ns-base:line:v2} 
\If{|A| = 0} break\EndIf \label{algo:ns-base:line:breakA} %\Comment{failed, early exit}
\State $v_2 \gets$ \Call{sample}{$A$} \Comment{\hlg{sample} node $v_2$ from set $A$} \label{algo:ns-base:line:sample-v2} 
\State $B \gets$ $N(v_0) \cup N(v_2)$ - \{$v_0, v_1, v_2$\} \Comment{\hlg{set union and difference}} \label{algo:ns-base:line:v3} 
\If{|B| = 0} break\EndIf \label{algo:ns-base:line:breakB} %\Comment{failed, early exit}
\State $v_3\gets$ \Call{sample}{$B$}  \Comment{\hlg{sample} node $v_3$ from set $B$} \label{algo:ns-base:line:sample-v3}
%\State VertexSet vs4 = $N(v_1)$ - $vs02$
\If{edge $(v_0, v_3)$ exist in \dg} \Comment{check closure}
\State $\alpha \gets m * |A| * |B| / 16$  \Comment{scaling factor}
\EndIf
\EndFor
%\State $C' = \sum C_i / N_s$ is the estimated count  \label{algo:ns:line:average}
\end{algorithmic}
\end{algorithm}
\begin{algorithm}[htb]
%\scriptsize
\footnotesize
\caption{Exact {\tt 4-cycle} counting in GraphZero~\cite{GraphZero}}
\label{algo:graphzero-4cycle}
\begin{algorithmic}[1]
  \For{{\bf each} vertex $v_1 \in$ \vs }  \Comment{\hlg{match $v_1$ to $u_1$}} \label{algo:dfs:for1}
    \For{{\bf each} vertex $v_2 \in$ \adj($v_1$)} \Comment{\hlg{match $v_2$ to $u_2$}} \label{algo:dfs:for2}
	  \If{$v_2\ge v_1$} break; \Comment{\hlg{symmetry breaking}} \label{algo:dfs:break1}
	  \EndIf
        \For{{\bf each} vertex $v_3 \in$ \adj($v_1$)} \Comment{\hlg{match $v_3$ to $u_3$}} \label{algo:dfs:for3} 
	  \If{$v_3\ge v_2$} break; \Comment{\hlg{symmetry breaking}} \label{algo:dfs:break2}
	  \EndIf
	  %\State $W \leftarrow$ \adj($v_1$) $\cap$ \adj($v_2$); \Comment{\hlg{set intersection: buffered in $W$}} \label{algo:dfs:buffer}
      %\For{{\bf each} vertex $v_3 \in W$} \Comment{\hlg{match $v_3$ to $u_3$}} \label{algo:dfs:for3}
      \For{{\bf each} vertex $v_4 \in $ \adj($v_1$) $\cap$ \adj($v_2$)} \Comment{\hlg{match $v_4$ to $u_4$}} \label{algo:dfs:for4}
	      \If{$v_4\ge v_0$} break; \Comment{\hlg{symmetry breaking}} \label{algo:dfs:break3}
	      \Else $ $ count ++; \Comment{\hlg{do the counting}}
	      \EndIf
	    \EndFor
	  \EndFor
    \EndFor
  \EndFor
\end{algorithmic}
\end{algorithm}

%\subsection{Helper Functions} \label{subsect:api-functions}
%\cref{listing:code-api} lists the helper functions in our system to help the user quickly implement a sampling scheme.

%\input{code-API}

\subsection{Stability of Error Prediction} \label{subsect:more-stability}

Figures ~\cref{fig:stable-estimated-error-friendster} and ~\cref{fig:stable-estimated-error-twitter} show the predicted errors in our convergence detection mechanism on \texttt{Fr} and \texttt{Tw} respectively when the pattern is \texttt{4-clique}.

\begin{figure}[h]
\centering
\includegraphics[width=0.38\textwidth]{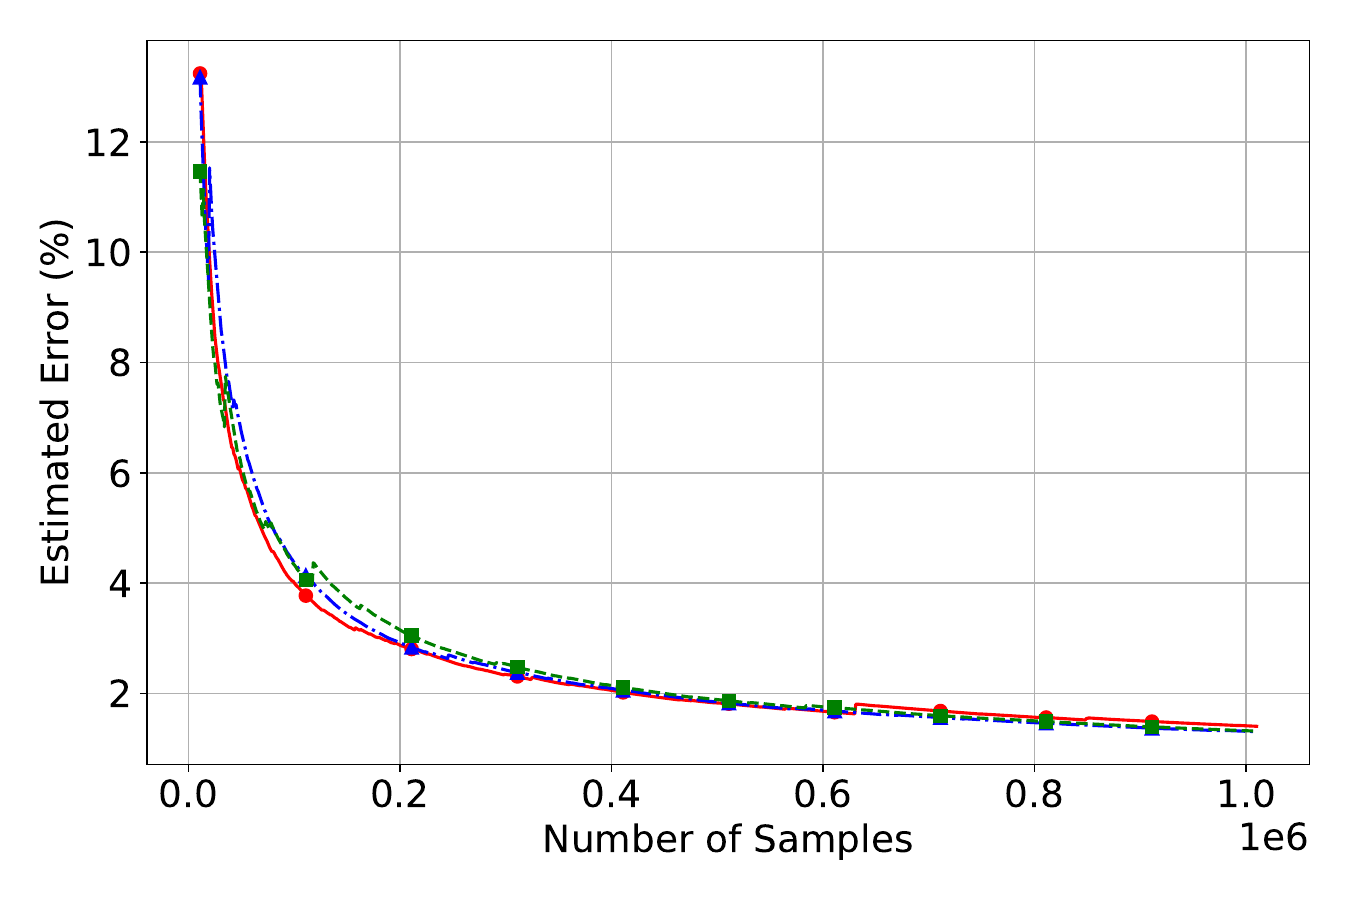}
\caption{Predicted errors in our convergence detection mechanism across three different runs (\texttt{4-clique} on \texttt{Fr}) are extremely stable.}
\label{fig:stable-estimated-error-friendster}
\end{figure}

\begin{figure}[b!]
\centering
\includegraphics[width=0.38\textwidth]{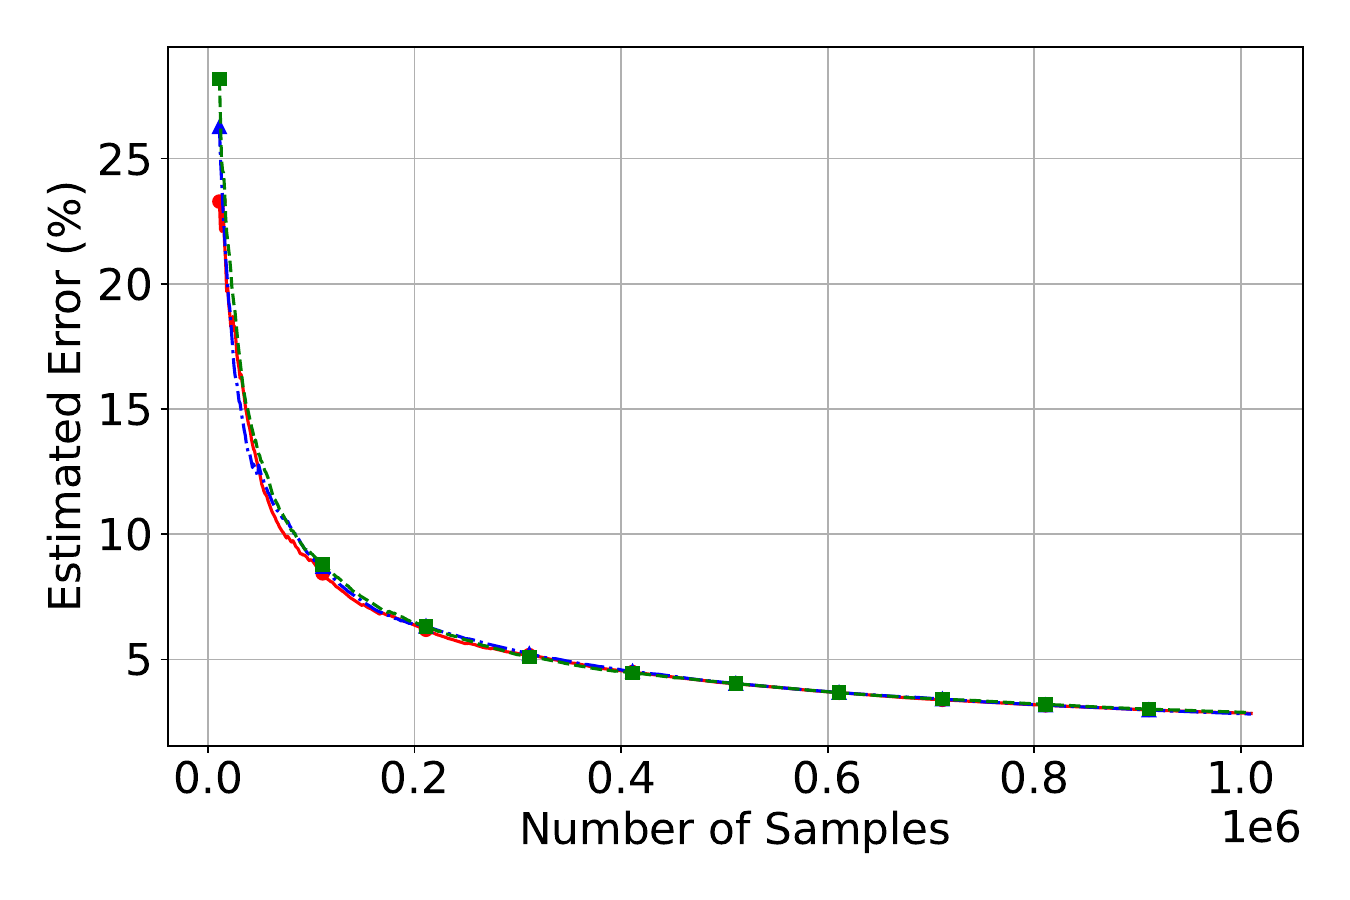}
\caption{Predicted errors in our convergence detection mechanism across three different runs (\texttt{4-clique} on \texttt{Tw}) are extremely stable.}
\label{fig:stable-estimated-error-twitter}
\end{figure}
